# Supplementary material for: Neural Mesh Refiner for 6-DoF Pose Estimation
Source: arXiv:2003.07561 source file (2020-03-26)
Supplement: Supplementary file 1 [file Appendix.tex]

\section*{Appendix}

\subsection{Enforcement of Quaternions to one hemisphere}\label{app:quaternions}
%\subsection{Enforcement of Quaternions to one hemisphere}
% http://planning.cs.uiuc.edu/node151.html
Let $ {\mathbb{Q}}$ represents the set of quaternions, in which each quaternion, $ \textbf{q} \in {\mathbb{Q}}$, is represented as $ \textbf{q} = a + b i + c j + dk$, and $ a,b,c,d \in {\mathbb{R}}$. A quaternion can be considered as a four-dimensional vector. The symbols $ i$, $ j$, and $ k$ are used to denote three ``imaginary'' components of the quaternion. The following relationships are defined: $ i^2 = j^2 = k^2 = ijk = -1$, from which it follows that $ i j = k$, $ j k = i$, and $ k i = j$.

The quaternion $\textbf{q}$ and $-\textbf{q}$ represent the same rotation because a rotation of $\theta$ in the direction $v$ is equivalent to a rotation of $2\pi-\theta$ in the direction $-v$.
One way to force uniqueness of rotations is to require staying in the ``upper half'' of $ {\mathbb{S}}^3$. For example, require that $ a \geq 0$, as long as the boundary case of $ a = 0$ is handled properly because of antipodal points at the equator of $ {\mathbb{S}}^3$. If $ a = 0$, then require that $ b \geq 0$. However, if $ a=b=0$, then require that $ c \geq 0$ because points such as $ (0,0,-1,0)$ and $ (0,0,1,0)$ are the same rotation. Finally, if $ a=b=c=0$, then only $ d=1$ is allowed.

\subsection{Projective Distance Estimation}\label{app:trans_geometric}

Fig.~\ref{fig:Geometric_trans} illustrates the projective distance estimation via geometric method which were adopted in previous state-of-the-art methods~\cite{sundermeyer2018implicit, kehl2017ssd, 6dposedobmvc2018}.
For each object we precomputed the 2D bounding box and centroid. To this end, the object is rendered at a canonical centroid distance $z_r$ ($z_r$ should be set larger than the object length in longitudinal axis so that the entire object can be projected onto the image plane). Subsequently, the object distance $z_s$ can be inferred from the projective ratio according to $z_s = \frac{l_r}{l_s}z_r$, where $l_r$ denotes diagonal length of the precomputed bounding box and $l_s$ denotes the diagonal length of the predicted bounding box on the image plane. Given its depth component $z_s$, the complete translational vector can be recovered geometrically as:
\begin{equation*}
x_s = \frac{(u - c_x) z_s}{f_x}, y_s = \frac{(v-c_x) z_s}{f_y}
\end{equation*}
where $[u, v]$ is the bounding box centre, and the matrix $[f_x,0,c_x; 0, f_y, c_y; 0, 0, 1]$ is the camera intrinsic calibration matrix. The formulation assumes that: (i) the object centre in 3D will be projected to the object bounding box in the 2D image; (ii) the predicted object class and rotation vector is correctly estimated.

\begin{figure}[h]
        \centering
        \includegraphics[width=0.45\textwidth]{figures/geometric_trans_2.png}
        \caption{Projective Distance Estimation.}
        \label{fig:Geometric_trans}
\end{figure}

%\subsection{Prove of extreme gradient of embedded Gaussian in non-local operations (*)}\label{app:weight_non_local}
%This phenomenal was also observed in another related work of~\cite{vaswani2017attention}.
%Our derivation mainly follows~\cite{he2015delving}.
%
%\noindent \textbf{Forward Propagation Case.}
%
%\noindent \textbf{Backward Propagation Case.}
